# Supplementary material for: FeatNavigator: Automatic Feature Augmentation on Tabular Data
Source: arXiv:2406.09534 source file (2024-06-13)
Supplement: Supplementary file 1 [file 9_appendix.tex]

\section{Appendix}
\label{sec:appendix}

\begin{lemma}
\label{lm.expectation_variacnce}
If a random variable x, s.t. \( -1 < x < 1, E(x)=0, Var(x) \leq \epsilon < 1 \), then \( 0 \leq E(|x|) \leq 2\sqrt{\epsilon} \) and \( 0 \leq Var(|x|) \leq \epsilon \).
\end{lemma}

\vspace{-10pt}

\begin{proof}
To begin with, we have 
\begin{equation}
E(x^2) = Var(x) - E(x)^2 \leq \epsilon.
\label{eq.lm.expectation_variance.1}
\end{equation}
Let $a$ be a constant \( 0 < a < 1 \), and we have \( E(|x|)=E(\sqrt{x^2}) \). For \( a<|x|<1 \), we have \( \sqrt{x^2}<\frac{1}{a}x^2 \), and for \( 0 \leq |x| \leq a \), we have \( \sqrt{x^2} \leq a \). Consequently, \( \sqrt{x^2} \leq a+\frac{1}{a}x^2 \). Thus for $E(|x|)$, we have
\begin{equation}
\label{eq.lm.expectation_variance.2}
\begin{aligned}
E(|x|)  & \leq E(a+\frac{1}{a}x^2) = a+\frac{1}{a}E(x^2). \\
\end{aligned}
\end{equation}

Based on Equations~\ref{eq.lm.expectation_variance.1} and~\ref{eq.lm.expectation_variance.2}, we have 
\begin{equation}
\label{eq.lm.expectation_variance.3}
E(|x|) \leq a+\frac{1}{a}\epsilon. \\
\end{equation}

In Equation~\ref{eq.lm.expectation_variance.3}, let \( a=\sqrt{\epsilon} \), we have \( E(|x|) \leq 2\sqrt{\epsilon}\). For $Var(|x|)$, we have
\begin{equation}
\begin{aligned}
Var(|x|) & = E(|x|^2)-E(|x|)^2 \leq E(|x|^2), \\
         & = E(x^2) \leq \epsilon. \\
\end{aligned}
\end{equation}

Given that \( 0 \leq E(|x|) \) and \( 0 \leq Var(|x|) \), we prove that \( 0 \leq E(|x|) \leq 2\sqrt{\epsilon} \) and \( 0 \leq Var(|x|) \leq \epsilon \).
\end{proof}
